# Supplementary material for: Tiny Machine-Learning Operations within Cyber-Physical Systems: a Field Study
Source: arXiv:2606.20952 source file (2026-10-24)
Supplement: Supplementary file 1 [file appendix.tex]

% === Appendix (online supplemental material) ===
% Uses IEEEtran's native \appendices (declared in main.tex); no extra package.

\section{Kaskasi II Trenching Intervals}
\label{app:kaskasiIntervals}
\input{App/1_kaskasiIntervals}

\section{Kaskasi II Soil Layer Identifiers}
\label{app:kaskasiSoilLayers}
\input{App/2_kaskasiSoilLayers}

\section{AFT Cable Guide Load Peak Classification - Kaskasi}
\label{app:loadPeaks}
\input{App/3_loadPeaks}

\section{Fitted Coefficients for Soil Layer Proportions}
\label{app:fittedCoefficientsSoilLayers}
\input{App/08_soilDensityCohesivenessParameters}

\section{AFT Cable Guide Load Peak Classification - South Fork}
\label{app:loadPeaksSouthFork}
\input{App/08_LoadPeaksSouthFork}

\section{South Fork Soil Layer Identifiers}
\label{app:southForkSoilLayers}
\input{App/08_southForkSoilLayers}
